# Supplementary material for: Optimizing NILC Extractions of the Thermal Sunyaev-Zeldovich Effect with Deep Learning
Source: arXiv:2402.00167 source file (2024-01-31)
Supplement: Supplementary file 1 [file Appendix.tex]

\appendix
\section{Individual Surface Brightness Profiles}
\begin{figure}[t!]
%http://localhost:8888/notebooks/Desktop/RESEARCH/RESOLVED_GROUPS_new/tully/code/individual_plots_groups_extraction.ipynb
\centering
    \includegraphics[width=0.95\textwidth]{figures/groups_block1_latex.pdf}%
    
    \includegraphics[width=0.37\textwidth]{figures/groups_block2_latex.pdf}
    
    \caption{Individual SZ surface brightness profiles. Red triangles, green diamonds, and black squares represent the profiles from PR2NILC, PR3NILC, and PR4NILC respectively. Uncertainties are shown only for PR4NILC and were estimated locally depending on the size and location of the extraction annulus (see \autoref{sec:uncertainty}). The PCG identification represents the objects in \autoref{tab:sample_info}; the corresponding BCG IDs are provided as well. Blue lines indicate the $1^{\circ}$ scale for each object.}%
    \label{fig:individual}%
\end{figure}
%%%%%%%%%%%%%%%%%%%%%%%%%%%%%%%%%%%%%%%%%%%%%%%%%%%%%%%%%%%%%%%%%
\newpage
\section{Weighted Average Stacked Profile}
\label{sec:weighted_avg}

\textbf{Stacking signals together is only acceptable when the spread about the mean is modest, and so one must search for possible for outliers that may be skewing the resulting stack. For the sample in this work, the two most massive systems were the closest in distance. One might expect the combination of their high masses and close distances to yield high S/N values, which could potentially bias the weighted stack. We tested this possibility by splitting our galaxy group sample into
low-mass (8 least massive) and high-mass (2 most massive) sub-samples. (We did not consider the bootstrapping method for the sub-samples due to insufficient sample size of the high-mass objects.)}

\textbf{The stacked profile from the full, low-mass, and high-mass samples are shown in \autoref{fig:weighted_avg}. Tenuous evidence points to a steeper profile for the high-mass sample compared to the low-mass sample within R$<$\Rvir; however, the data were mostly consistent within the uncertainties. In addition, both sub-samples exhibited a bump feature near 1.75 \Rvir, meaning the bump was not dominated by only low- or high-mass systems.}

\begin{figure}[h!]
%http://localhost:8888/notebooks/Desktop/RESEARCH/RESOLVED_GROUPS_new/tully/code/individual_plots_groups_extraction.ipynb
\centering
    \includegraphics[width=0.75\textwidth]{figures/stacked_groups_split.pdf}%

    \caption{Weighted average stacked profiles using the full (blue squares), low-mass (orange triangles), and high-mass (purple diamonds) samples. The data are slightly offset on the horizontal axis for clarity; the blue and orange data are shifted to the left and the right of each purple diamond respectively. The weighted stack was calculated using the empirical variance estimated for each local field. The low-mass sample does not show a value for the innermost bin because it was smaller than the 20' exclusion radius (i.e., 0.25 R$_{500} < 20^{\prime}$).}%
    \label{fig:weighted_avg}%
\end{figure}
